# Supplementary material for: Remote Observation of Field Work on the Farm
Source: arXiv:2103.03163 source file (2021-03-04)
Supplement: Supplementary file 1 [file additionalResourcesBudget.tex]

\newpage
\section{Additional Resources, Budget and References} 
\textit{Describe all resources available to carry out the project including collaborative relationships and additional funding sources.} %(do not include dollar amounts). CIDA funding is intended to be of limited duration and the objective is to position faculty to compete successfully for a long-term extramural funding.  Indicate the source(s) of extramural funding you anticipate seeking as long term for the project.

Project funding to date for this project has come from PI Ju's start-up funds, from 2019 research gift funding from Accenture intended to support human-robot teaming, as well as in-kind contributions from PI Willett's research staff. No additional research funding resources are available for the period we are applying for CIDA RIF. 

The goal of this RIF research will be to build up enough pilot data and preliminary results to apply for National Robotics Initiative or equivalent funding in the 2021 and 2022 funding cycles.

\section{Budget rationale} \textit{Provide a justification for your budget.  Be sure to explain any requests for large equipment or supplies/services.}

\vspace{1em}
%\begin{table}[h]
\begin{tabular}{llll}
Year 1     & Description  & Itemized Amount & Category Total \\
\hline
Salary  &     &     &    \\
Graduate Student Support & 1 AY PhD   & 67,685  & 67,685 \\
Equipment  &     &  &  \\
Supplies   & remote interactive streaming setup & 5,000 & 5,000 \\
Services   &  mobile service  & 1,000 & 1,000 \\
Travel     & 3 trips for PIs and student to farm & 1,300 & 1,300 \\
\hline
Total      &     &  \$74,985  &   \$74,985            
\end{tabular}
%\end{table}
\vspace{2em}

%\begin{table}[h]
\begin{tabular}{llll}
Year 2     & Description  & Itemized Amount & Category Total \\
\hline
Salary  &     &     &    \\
Graduate Student Support & 1 AY PhD   & 69,070  & 69,070 \\
Equipment  &     &  &  \\
Supplies   & remote interactive streaming setup & 3,500 & 3,500 \\
Services   &  mobile service & 1,000 & 1,000 \\
Travel     & 3 trips for PIs and student to farm & 1,300 & 1,300 \\
\hline
Total      &     &  \$74,870    &   \$74,870            
\end{tabular}
%\end{table}

\vspace{2em}

One Information Science PhD student will be funded for academic year research to develop tools, conduct remote ethnography, perform analysis, and write documentation. Support includes GRA, tuition, and insurance.

Supplies for the remote interactive streaming setup include expenses for chemical sensors, mobile phones, mobile hotspots, charging equipment, and cables, as well as mounting and housing equipment. We anticipate that we will another set of phones to enable greater coverage for our research apparatus in year 2, but that we will be able to get the same model as used in year 1, used.

Ten months of pay-as-you-go mobile data service is needed for 2 data plans. (Data is not needed for the winter months of November and December.)

Travel for three trips annually for the PIs and the graduate student to make an on-site visit to the farm near Buffalo, NY to help set up equipment, communicate with farmers and farm workers, and to capture the context for the research.
